# Supplementary material for: Zero-shot Model Diagnosis
Source: arXiv:2303.15441 source file (2023-03-27)
Supplement: Supplementary file 1 [file appendix_sectionD.tex]

\section{Metric Evaluation}
\subsection{Image synthesis quality}
Unconstrained synthesis of counterfactual examples will result in image generation collepse. \ourmodel’s loss constraint helps to avoid exaggerated semantic variation. This section evaluates the generated image quality from both quantitative and qualitative perspectives.

Decomposing the latent space of StyleGAN has been well studied in recent years. \ourmodel adopts the principle from StyleSpace \cite{2021stylespace} to locate and filter effective attribute-oriented channels. To validate the reliability of approach, we replace this component with different alternatives including optimization (1) along SeFa axis \cite{2021sefa}, (2) within $\mathcal{Z}$ space \cite{Li_2021_CVPR}, or (3) within $\mathcal{W}$ space. We compare the visual sanity of the generated counterfactual. The tables show that \ourmodel image quality is finer under both PSNR (Peak Signal to Noise Ratio) and SSIM (Structured Similarity Indexing Method) \cite{SSIM} metrics. 

%  evaluate the perceptual quality for counterfactual examples generated by \ourmodel and StylEx \cite{Lang_2021_ICCV}.
\begin{table}[h]
  \centering
  \caption{Image synthesis quality. The table shows that \ourmodel supports fine-grained synthesis with our choice of searching space.}
  \begin{tabular}{@{}lcccc@{}}
     \toprule
     Method & Constrain & PSNR  &  SSIM \\
     \midrule
     $\mathcal{W}$ space & $L_2$                                   & ???\% & ???\%\\
     $\mathcal{Z}$ space \cite{Li_2021_CVPR}  & $L_2$                & ???\% & ???\%\\
     SeFa axis \cite{2021sefa}  &$L_{\infty}$                 &  ???\% &  ???\%\\ 
     AttGAN \cite{attGAN}  &$L_{\infty}$                 &  ???\% &  ???\%\\ 
     \ourmodel &$L_{\infty}$                                 &  ???\% &  ???\%\\
     \bottomrule
  \end{tabular}
  \label{tab:image_quality}
\end{table}
